# Supplementary material for: Explainable Action Advising for Multi-Agent Reinforcement Learning
Source: arXiv:2211.07882 source file (2023-06-16)
Supplement: Supplementary file 1 [file appendix_A.tex]

\section{Code}

We have attached our code in the supplementary material, under the directory of ``EAA\_22nips''. 

In this directory, we follow the requirements on publishing the research code that we provide the scripts of training, evaluation, per-trained saved model, environment requirement and the command to produce the result in README.

Notice that to see the performance of what we show in the manuscript, continuing training on a saved model is the easiest way to see it. The initial test performance result printed in the terminal before the agents get further training gives its performance. See README what the command is in the Quick Start Section.

We have provided the procedure to run the full experiments as well, i.e. everything trained from scratch. Any MARL model during training will be saved to the directory of ``model'' and the data such as episode rewards of evaluation is saved to the directory of ``publish\_results''. All the parameters with respect to the experiment is provided in the file of ``experiment\_parameters''. If you wish to change the teacher model, modify ``teacher\_rnn\_path'' in it. Notice that for running VIPER, there is no model you need to save but a dataset that the algorithm generates for training the DT. See README for details in the Full Experiments Section.  

We have provided the result data that we generate plots, and the scripts accordingly in the directory of ``draw\_plots''. From the root directory when each of the script is called, it generates the result plots in our submission.
