# Supplementary material for: Explainable Action Advising for Multi-Agent Reinforcement Learning
Source: arXiv:2211.07882 source file (2023-06-16)
Supplement: Supplementary file 2 [file appendix_B.tex]

\section{The Full Version of Algorithm}
\subsection{Explainable Action Advising}

\begin{algorithm}[h!]
\caption{Explainable Action Advising}
\label{alg:algorithm}
\textbf{Input}:  Teacher policies $\pi_1^*, \pi_2^*... \pi_n^*$ for the $n$-agent mission, heuristic function $h$ \\
\textbf{Parameter}: Advice budget $b$, advice decay rate $\gamma$\\
\textbf{Output}: Students policies. $\pi_1$... $\pi_n$ 
\begin{algorithmic}[1] 
\FOR{$i = 1...n$} \label{start setup}
    \STATE Expert DT policy $\hat{\pi_i^*} = VIPER( \pi_i^*)$ \label{use viper to constuct}
    \STATE Memory $M_i = \phi$
    \STATE In-memory sub-tree DT policy $\pi_i' = \phi$
\ENDFOR
\STATE Budget of advice left $x=b$ \label{end setup}
\STATE Initialize students policies $\pi_1 ... \pi_n$
\STATE Iter $j=0$
\WHILE{j  $ \leq max\_iter$}
    \STATE $t=0, D = \emptyset$
    
    \WHILE{$episode\_not\_end$}
        \FOR{$i = 1...n$}
            \STATE $a = \pi_i'(s^0 ... s^t)$ \label{core start}
            \IF{$a != null$ and $\gamma^j < \alpha \sim \mathcal{U}(0,1)$} \label{follow sub-tree 1}
                \STATE $a_i^t = a$ \label{follow sub-tree 2}
            \ELSE
                \IF {$x > 0$ and $h(s^t)$} \label{ask teacher creteria}
                    \STATE $x = x-1$ \label{decrease budget}
                    \STATE $a_i^t = \pi_i^*(s^t)$ \label{use teacher action}
                    \IF {$a_i^t == \hat{\pi_i^*}(s^0 ... s^t)$ and $P(a_i^t | \hat{\pi_i^*}, s^0 ... s^t) > threshold$} \label{add path creteria}
                        \STATE $M_i$.add\_DT\_path($\hat{p}^t_i = \text{path} (\hat{\pi_i^*}, s^0 ... s^t)$) \label{add path}
                    \ENDIF
                \ELSE
                    \STATE $a_i^t = \pi_i(s^t)$ \label{core end}
                \ENDIF
            \ENDIF
            \STATE $D = D \cup (s^t, a_i^t, \mathcal{R}(s^t, a_i^t))$ \label{collect data}
        \ENDFOR
        \STATE $t = t + 1$ 
    \ENDWHILE
    
    \STATE $\pi_1 ... \pi_n = $ student.train($D$) \label{student train}
    \STATE $\pi_1' ... \pi_n'$ = update\_tree($M_1$) ... update\_tree($M_n$) \label{update tree}
    \STATE $j = j + 1, p = \gamma ^ j$ \label{update iter}
\ENDWHILE
\STATE \textbf{return} solution
\end{algorithmic}
\end{algorithm}

%%%%%%%%%%%%%%%%%%%%%%
The full algorithm of EAA is shown in Algorithm \ref{alg:algorithm}. Same as the outline version that is provided in the manuscript, it takes in a set of pre-trained MARL policies $\pi_1^*, \pi_2^*... \pi_n^*$ as the teacher for the  $n$-agent mission (one for each agent $i$), and a function $h$ that determines when the advice should be issued to a student agent. Two parameters are needed: an advising budget $b$ and decay rate $\gamma$. The advising budget is limited to $b$, and students will not receive any additional advice after $b$ pieces of advice have been issued. The advice decay rate $\gamma$ determines the likelihood that the student reuses advice when selecting actions. For further information, please see the main manuscript.
%Discussion on the functionalities are referred to the outline version.

Lines \ref{start setup} to \ref{end setup} contain the detailed setup steps. For each RL teacher policy $\pi_i^*$, first VIPER is used to distill an appropriate decision tree (DT) policy $\hat{\pi_i^*}$ that represents it (line \ref{use viper to constuct}). Then in the next 2 lines each student is assigned a memory $M_i$ for further data collection, and an empty DT $\pi_i'$ that will grow to reconstruct a partial teacher policy as a 
sub-tree. We also set the counter of budget left $x$ and initialize the student policies $\pi_i$. 

The core of the algorithms lies between lines \ref{core start} and \ref{core end}. For each episode, each time step and each agent, given the states in the current episode $s^0 ... s^t$, we first query the sub-tree DT in memory $\pi_i'$ (line \ref{core start}). This means the student may reuse the action advice that it generalizes from the previous advice taken. Note that for implementation where the input of the policy is a single current state, we only need to give $s^t$. Since $\pi_i'$ is a sub-tree of $\hat{\pi_i^*}$, its output $a$ will be either the same as $\hat{\pi_i^*}$ or undecided, i.e. $null$, if the advised action of the current state features has not been stored. Additionally, the student may gradually forget the stored advice, and thus the advice is only taken with probability of $\gamma^j$. This probability becomes smaller when the student is trained further and less reliant on the stored advice. 

Secondly, we consider the case where the student has not previously received relevant advice. If there is still advising budget $x$ left, and $h$ determines it is appropriate to give advice (line \ref{ask teacher creteria}), the budget counter decreases and the student takes the teacher's action $\pi_i^*(s^t)$ (line \ref{decrease budget}, \ref{use teacher action}). Next, in line \ref{add path creteria}, we check if the teacher's action advice is equal to the action given by the VIPER DT policy $\hat{\pi_i^*}$. We make this optional check because a discrepancy might exist in equivalent policies due to randomness in states that the teacher does not have a high probability on any of the action but rather distributed evenly on the action set. This is omitted but motivated in the outline version that we only want to collect the advice with a filter of higher quality. Therefore, only if both of them agree on this action advice, and $\hat{\pi_i^*}$ predicts this action has a probability higher than the $threshold$, then the memory $M_i$ collects this DT path $\hat{p}^t_i$ given by $\hat{\pi_i^*}$ (line \ref{add path}) and the state history (for Markovian case, only input $s^t_i$ is sufficient). In this way, only the key actions and reasons are preserved. 

Lastly, if no advised action is available, the student simply explores and exploits the environment as  trained normally by its algorithm
(line \ref{core end}). Episode data is collected for training the student's policy (line \ref{collect data}, \ref{student train}), while episode information is updated (line \ref{update iter}). The algorithm of updating the tree (line \ref{update tree}) is presented in the next section.
Note that our algorithm does not assume full observability of the state for agents. Similar to the settings of some MARL algorithms, partial observability is a special case and for notational simplicity we follow the convention using (state, action) pairs.

%%%%%%%%%%%%%%%%%%%%%%%%%%%%%%%%%%%%%%%%%%%%%%%%%%%%%%
% sub sections for the helper functions or components.
\subsection{Update In-memory Sub-tree}

\begin{algorithm}[h!]
\caption{Update In-memory Sub-tree}
\label{alg:algorithm_update_memory}
\textbf{Input}: $m$ DT paths $p_{il}$ in memory $M_i$ of student $i$, previous Sub-tree DT policy $\pi_i'$ \\
\textbf{Output}: Updated $\pi_i'$
\begin{algorithmic}[1] 
\FOR{$l = 1...m$} 
    \STATE $\{u_0, u_1...u_{d-1}\} = p_{il}$
    \STATE $k = 0$
    \WHILE{$u_k \in \pi_i'.nodes$} \label{find existing nodes1}
        \STATE $k = k + 1$
    \ENDWHILE \label{find existing nodes2}
    \WHILE{$k < d$} \label{add child1}
        \STATE $\pi_i’$.add\_child($u_{k-1}, u_k, u_k.inequality$)
        \STATE $k = k + 1$
    \ENDWHILE \label{add child2}
\ENDFOR
\end{algorithmic}
\end{algorithm}

Let us assume that there have been $m$ collected DT paths $p_{il}$ in memory $M_i$ where $l = 1...m$. 
Each of them is a list of nodes $\{u_0, u_1...u_{d-1}\}$ where $d$ is the depth of the leaf node that outputs 
a probability on action.
Each pair of adjacent nodes $(u_{k-1}, u_{k}) \forall{k} \in [1, d-1]$ has a relation of (parent, child), with $u_0$ as the root.
We use a standard DT structure such that node $u_k$ contains information of $parent, inequality\_sign, value$ etc.  

Algorithm \ref{alg:algorithm_update_memory} updates the in-memory sub-tree policy $\pi_i'$.
As the paths in $M_i$ and $\pi_i'$ both originate from the same tree -- the teacher's $\hat{\pi_i^*}$ -- there will be no conflicts when merging.
Therefore, for each path $\{u_0, u_1...u_{d-1}\}$, it first finds the node $u_k$ that does not exist in $\pi_i'$ (lines \ref{find existing nodes1} to \ref{find existing nodes2}). 

This implies the remaining nodes in the branch also do not exist in $\pi_i'$.
Thus by locating the top-most node in the path that does not exist in $\pi_i'$, 
we can directly add the rest of the branch according to the inequality signs of DT (DT inequality signs decide the index of branch, e.g. left/right child in binary DT), as shown in lines \ref{add child1} to \ref{add child2}.
