# Supplementary material for: Explainable Action Advising for Multi-Agent Reinforcement Learning
Source: arXiv:2211.07882 source file (2023-06-16)
Supplement: Supplementary file 3 [file appendix_C.tex]

\section{Additional Experiment}

\begin{figure}
    \centering
    \includegraphics[width=1\textwidth]{plots/ablation(1-dt+nn).pdf}
    \caption{A comparison of an ablated version of EAA which always takes the teacher's advice, EAA (Always Accept), to standard EAA when the teacher has access to both its original neural network policy and the extracted decision tree (DT + NN).}
    \label{fig:ablated-1}
\end{figure}

\begin{figure}
    \centering
    \includegraphics[width=1\textwidth]{plots/ablation(3-dt).pdf}
    \caption{A comparison of an ablated version of EAA which always takes the teacher's advice, EAA (Always Accept), to standard EAA when the teacher only has access to its extracted decision tree (DT).}
    \label{fig:ablated-3}
\end{figure}

In this section, we include an experiment in which we compare standard EAA to an ablated version which lacks the transfer learning check discussed in Sec.~\ref{subsection: Generalization and Transfer Learning}.
% ablated run without the ignoring mechanism that is omitted in the manuscript due to space limit.
The results are shown in Figure \ref{fig:ablated-1} and Figure \ref{fig:ablated-3}. 

% In both the cases where there are two teachers of DT + NN and only one teacher of DT, always accepting the advice from non-optimal teacher has a worse result that we have anticipated.
In both cases -- a DT + NN teacher and a DT-only teacher -- always accepting the advice from a non-optimal teacher performs worse than standard EAA.
The teacher is trained in an environment with no rubble, and thus when the student encounters a room with rubble, it is more advantageous for the student to execute an exploratory action rather than listening to the teacher, which happens in the standard EAA version.
In the (Always Accept) versions, this exploratory action is not taken and instead the student always accepts the teacher's (potentially non-optimal) advice, resulting in worse performance.
% The teacher is trained in an environment where there is no rubble, and thus with the ignore mechanism on features with rubble, the standard EAA performs better. 

For EAA-Early, the fact that always accepting advice is similar to standard EAA may be due to advice being given continuously resulting in the budget being used up at a very early stage.
This is similar to the Importance variant as the threshold for giving advice is rather low.
It can be observed that EAA is better at the beginning when it ignores non-optimal advice, but this effect is limited if the advice is given too densely in a limited period of time as in the Early variant.
We suspect that this is due to limited updates in the network parameters per iteration.
% The effect is not significant if advice is given too densely at the beginning, because the network parameters are only changed slightly so far and would not affect the performance too much. 

Instead, if the advice is given more sparsely, for example in EAA-Alternative, ignoring non-optimal advice has a more significant effect.
Empirically, the later the budget is used up the better the performance, something that is also seen in the Mistake Correcting variant.

In the ablated EAA version which always accepts advice, we notice that in some cases the student fails to converge to the optimal reward.
We conjecture that this occurs when the budget lasts a long time -- Alternative and Mistake Correcting variants -- which prevents the student from learning to converge to optimal on its own.
Additionally, the variance in the policy returns is quite a bit larger for the ablated versions -- again likely due to taking occasionally poor actions resulting in the policy being more likely to execute non-optimal sequences.
% With always accepting the non-optimal advice, some still converge to optimal while others not, because only when the parameters are trained in the wrong direction to a certain extent, when the teacher stops giving advice, the student might still learn to train themselves to converge to optimal.
% This contains randomness when calculating gradient descents due to the samples generated randomly, but the variance of always accepting non-optimal advice is much higher.

Moreover, removing the original policy NN from the teacher slightly improves the ablated EAA variants (Fig.~\ref{fig:ablated-3}).
When the teacher's advice is based solely off the extracted DT, the advice is more likely to be erroenous, which ironically means more likely to be correct if the initial advice was incorrect (as in this case).
So in a roundabout way, due to the lower quality advice from the teacher, the ablated version which always accepts advice ends up performing better than the ablated version in which the teacher has access to both its DT and NN policies.
% Moreover, removing the NN teacher makes always accepting non-optimal advice less worse. When NN teacher and DT teacher are both present, they give advice if they agree, and thus the advice is more certain, which means certainly optimal.
% Due to the lower quality, with NN teacher would have a worse effect.

% The results correspond to what we have expected.
