# Supplementary material for: Explainable Action Advising for Multi-Agent Reinforcement Learning
Source: arXiv:2211.07882 source file (2023-06-16)
Supplement: Supplementary file 4 [file appendix_D.tex]

\section{Room Layout}

\begin{figure}
    \centering
    \includegraphics[width=0.4\textwidth]{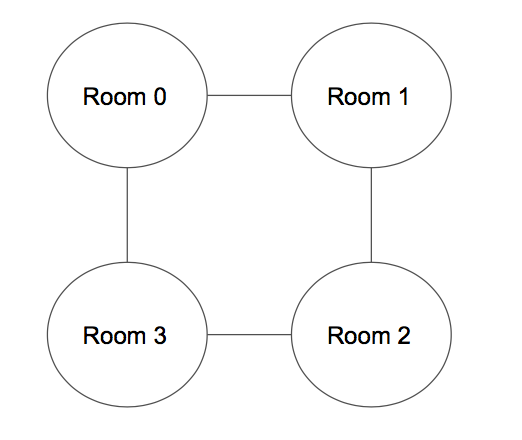}
    \caption{Graph of the 4 Room Layout}
    \label{fig:map_4_room}
\end{figure}

\begin{figure}
    \centering
    \includegraphics[width=0.7\textwidth]{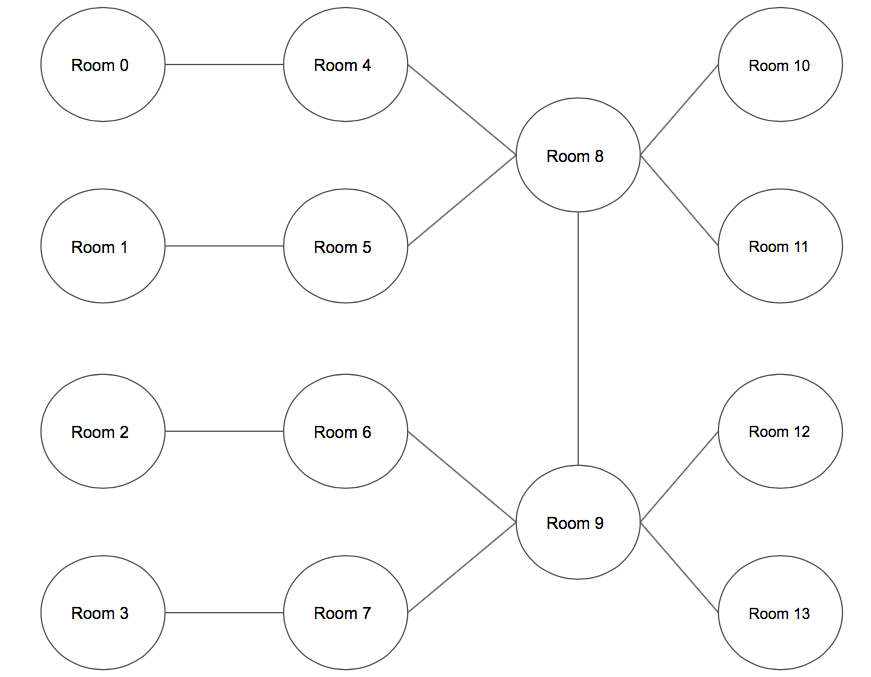}
    \caption{Graph of the 14 Room Layout}
    \label{fig:map_14_room}
\end{figure}

\begin{figure}
    \centering
    \includegraphics[width=0.4\textwidth]{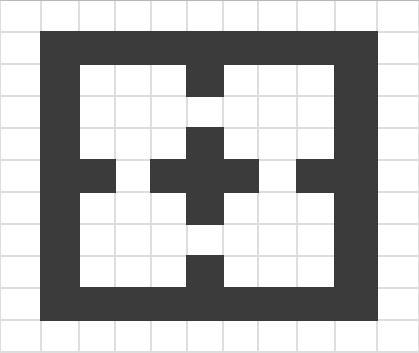}
    \caption{Grid of the 4 Room Layout}
    \label{fig:map_4_room_grid}
\end{figure}

\begin{figure}
    \centering
    \includegraphics[width=0.7\textwidth]{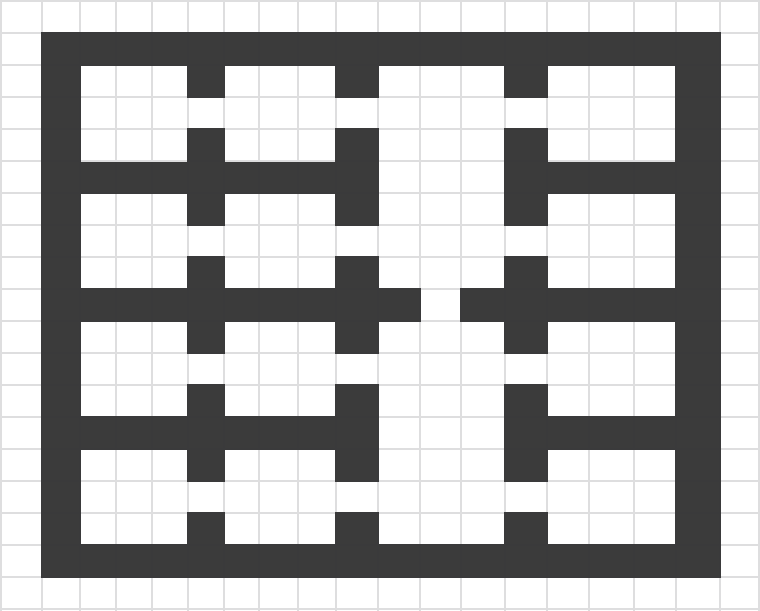}
    \caption{Grid of the 14 Room Layout}
    \label{fig:map_14_room_grid}
\end{figure}

We here present the graph maps of our environments of Four Room and Fourteen Room in Figure \ref{fig:map_4_room} and Figure \ref{fig:map_14_room}. The grid maps are in Figure \ref{fig:map_4_room_grid} and Figure \ref{fig:map_14_room_grid}.

In our scenario, the team is rewarded only when the medic has healed a victim, which may be hidden behind rubble and thus requires the engineer to remove. Rubble is scattered randomly in various rooms without replacement. The action set is meta-actions with respect to navigation, healing victims, and removing rubble (for the entire room). In the transfer learning experiments presented in the manuscript, the teacher is trained with the same room layout but without rubble (0 rubble, 1 victim), and is used to teach students who learn in the standard layout with rubble (3 rubble, 1 victim).
% Furthermore, the student trained with EAA in the no rubble environment performs better in the environment that is with rubble (3 rubble, 1 victim).
% ???
