# Supplementary material for: Explainable Action Advising for Multi-Agent Reinforcement Learning
Source: arXiv:2211.07882 source file (2023-06-16)
Supplement: Supplementary file 5 [file appendix_F.tex]

\section{Comparing various MARL Algorithms for Teacher and Student}

\begin{figure}
    \centering
    \includegraphics[width=0.95\textwidth]{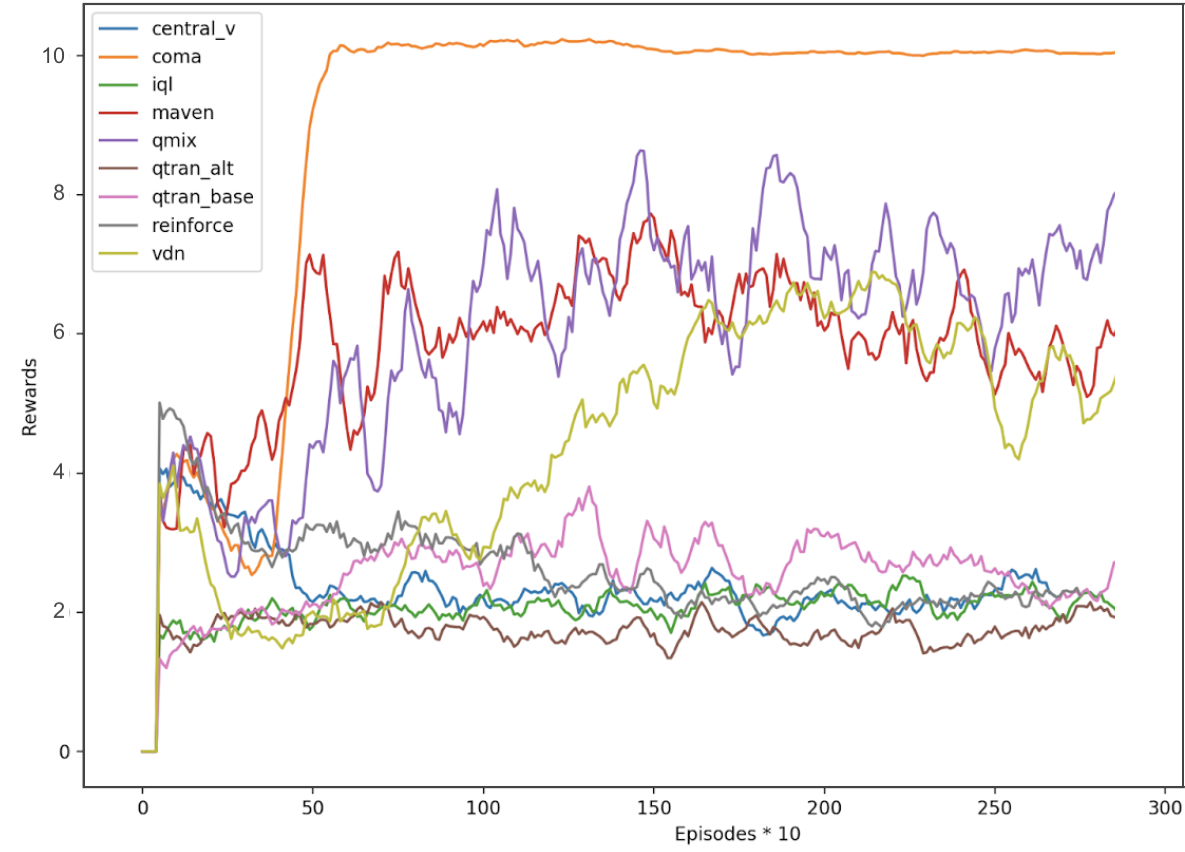}
    \caption{Performance of Various MARL algorithms}
    \label{fig:map_4_room}
\end{figure}

% In our main experiments our EAA algorithm is built upon the scenario where both the teacher and student are COMA team, because COMA serves especially well in our scenario where team members map from the belief over space to the actions.
In our main experiments, our EAA algorithm uses teacher and student policies trained with COMA, as initial experiments showed that COMA outperformed other common MARL algorithms for our scenario which maps a belief space to actions.
Although our focus is not to investigate MARL algorithm performance, here we provide an initial exploratory analysis indicating policy performance according to several common methods.
% Although picking what specific MARL algorithm is not our major focus, we here provide the initial exploratory analysis among various MARL algorithms.
This exploratory is done for the 4-room scenario described in our manuscript.
\begin{enumerate}
    \item (central\_v - CommNet) Learning Multiagent Communication with Backpropagation \cite{sukhbaatar2016learning}
    \item (coma) Counterfactual Multi-Agent Policy Gradients \cite{foerster2018counterfactual}
    \item (iql) Multiagent Cooperation and Competition with Deep Reinforcement Learning \cite{tampuu2017multiagent}
    \item (maven) MAVEN: Multi-Agent Variational Exploration \cite{mahajan2019maven}
    \item (qmix) QMIX: Monotonic Value Function Factorisation for Deep Multi-Agent Reinforcement Learning \cite{rashid2018qmix}
    \item (qtran\_alt) QTRAN: Learning to Factorize with Transformation for Cooperative Multi-Agent Reinforcement Learning \cite{son2019qtran}
    \item (qtran\_base) QTRAN: Learning to Factorize with Transformation for Cooperative Multi-Agent Reinforcement Learning \cite{son2019qtran}
    \item (reinforce - G2ANet) Multi-Agent Game Abstraction via Graph Attention Neural Network \cite{liu2020multi}
    \item (vdn) Value-Decomposition Networks For Cooperative Multi-Agent Learning \cite{sunehag2017value}

\end{enumerate}
