# Supplementary material for: Explainable Action Advising for Multi-Agent Reinforcement Learning
Source: arXiv:2211.07882 source file (2023-06-16)
Supplement: Supplementary file 6 [file appendix_E.tex]

\section{Structure and Hyper Parameters}

\begin{figure}
    \centering
    \includegraphics[width=0.5\textwidth]{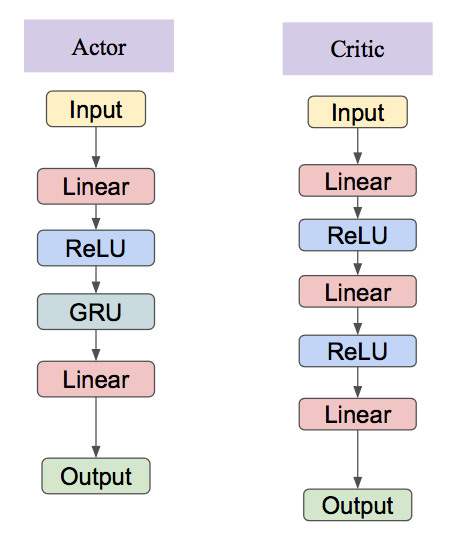}
    \caption{The structure of COMA}
    \label{fig:coma structure}
\end{figure}

We would like to provide the structure and hyper parameters of the COMA team that we use. For details, please see code. The neural network of the COMA team is shown in Figure \ref{fig:coma structure} which is composed of an actor and a critic network.

 \begin{tabular}{ |p{5cm}||p{3cm}|p{4cm}|  }
 \hline
 \multicolumn{3}{|c|}{Hyper Parameters} \\
 \hline
 Name & Value & Additional Notes \\
 \hline
Optimizer   & RMS    &    \\
Activation Function & ReLU  &    \\
Num Nodes Per Linear (Actor) & 64 & \\
Num Nodes Per GRU (Actor) & 64 & \\
Num Nodes Per Linear (Critic) & 128 & \\
Learning Rate (Actor) & 1e-4 & \\
Learning Rate (Critic) & 1e-3 & \\
Batch Size  &  32& \\
Epsilon & 0.5 &  \\
Gamma & 0.99 & \\
Evaluation Cycle &1000 & (For the demo experiment)  \\
Epochs   & 30000& (For the demo experiment)\\

 \hline
\end{tabular}\label{tmp}

% Critic Input Size  &  98& \\

A few common hyper parameters are shown in Table \ref{tmp}. See code ``common/arguments.py'' for others.
